# Supplementary material for: A Sober Look at LLMs for Material Discovery: Are They Actually Good for Bayesian Optimization Over Molecules?
Source: arXiv:2402.05015 source file (2024-05-28)
Supplement: Supplementary file 1 [file 99_apndx_notes.tex]

%!TEX root=../main.tex

\section*{Finding 1: Results with fixed features}

\begin{figure}[h!]
	\centering
	\includegraphics[width=0.5\linewidth]{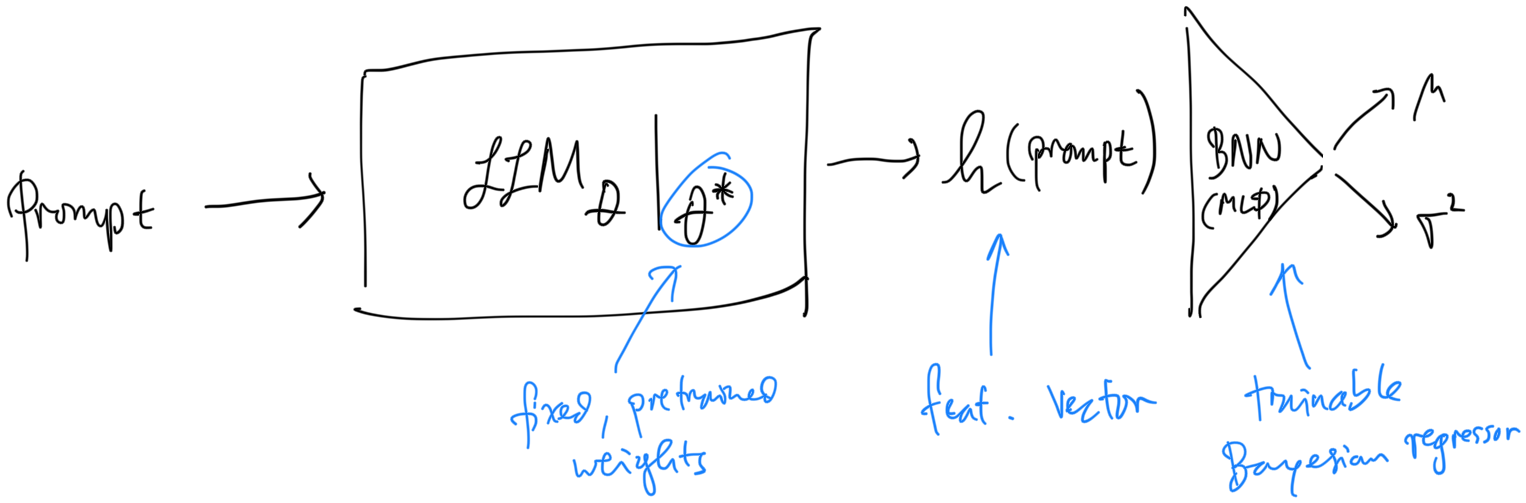}

	\caption{\textbf{Source of uncertainty:} The BNN regressor. Already more principled than the uncertainty of ICL.}
\end{figure}

Datasets:
\vspace{-1em}
\begin{itemize}
	\small
	\item \textbf{Redoxmer}: 1406 molecules, minimizing redox potential.
	\item \textbf{Solvation}: 1406 molecules, minimizing solvation energy.
\end{itemize}

Methods:
\vspace{-1em}
\begin{itemize}
	\small
	\item \textbf{RS}: random search
	\item \textbf{GP}: GP with the Tanimoto kernel
	\item \textbf{LA}: the Laplace-approximated MLP neural net
\end{itemize}

Foundation models/features:
\vspace{-1em}
\begin{itemize}
	\small
	\item \textbf{Fingerprints}: Molecular fingerprints baseline
	\item \textbf{Molformer}: Simple transformer over SMILES baseline
	\item \textbf{GPT2-M}: GPT2 Medium (345M params)
	\item \textbf{GPT2-L}: GPT2 Large (774M params)
	\item \textbf{Llama2-7B}: 7B params
	\item \textbf{T5-B}: T5-Base (220M params)
	\item \textbf{T5-B-Chem}: T5-B finetuned with chemistry data (220M params) \citep{christofidellis2023unifying}
\end{itemize}

Prompt types:
\vspace{-1em}
\begin{itemize}
	\small
	\item \textbf{just-smiles}: \emph{``\texttt{\{smiles\_str\}}''}
	      % \item \textbf{completion}: \emph{``The estimated redox potential of the molecule \texttt{\{smiles\_str\}} is: ''}
	      % \item \textbf{single-number}: \emph{``Answer with just numbers without any further explanation! What is the estimated redox potential of the molecule with the SMILES string \texttt{\{smiles\_str\}}?''}
\end{itemize}

Acquisition function: Thompson sampling---for a faithful assesment of the posterior.

\begin{figure}[h!]
	\centering

	\includegraphics[width=0.45\linewidth]{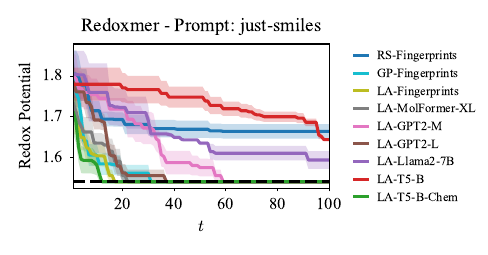}
	\includegraphics[width=0.45\linewidth]{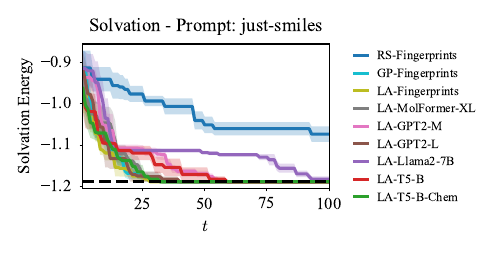}

	\caption{
		Fixed-feature performance, i.e.\ the LLM is frozen and train only the last regression layer.
		The acquisition function is Thompson sampling.
	}
\end{figure}

\begin{summarybox}
	Even when the LLM is fixed \& the prompt is naive, its features are very informative.
	However, this only holds for the chemistry-specific LLM.
\end{summarybox}

\clearpage

\section*{Finding 2: Effects of prompting}

\begin{figure}[h!]
	\centering
	\includegraphics[width=0.5\linewidth]{figs/diagram_fixed_feat}

	\caption{\textbf{Source of uncertainty:} The  regressor, via the Laplace approximation. Already more principled than the uncertainty of ICL.}
\end{figure}

Prompt types:
\begin{itemize}
	\item \textbf{just-smiles}: \emph{``\texttt{\{smiles\_str\}}''}
	\item \textbf{completion}: \emph{``The estimated redox potential of the molecule \texttt{\{smiles\_str\}} is: ''}
	\item \textbf{single-number}: \emph{``Answer with just numbers without any further explanation! What is the estimated redox potential of the molecule with the SMILES string \texttt{\{smiles\_str\}}?''}
\end{itemize}

\begin{figure}[h!]
	\centering

	\includegraphics[width=0.45\linewidth]{figs/redox-mer/fixed_feat_just-smiles-average}
	\includegraphics[width=0.45\linewidth]{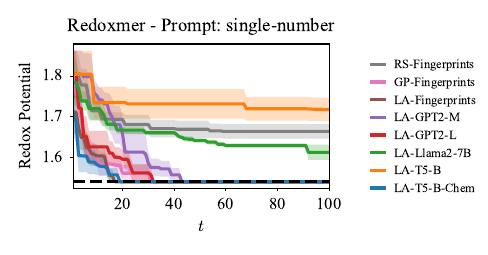}

	\includegraphics[width=0.45\linewidth]{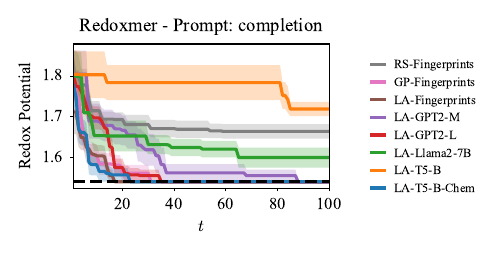}

	\vspace{-2em}
\end{figure}

\begin{figure}[h!]
	\centering

	\includegraphics[width=0.45\linewidth]{figs/solvation/fixed_feat_just-smiles-average}
	\includegraphics[width=0.45\linewidth]{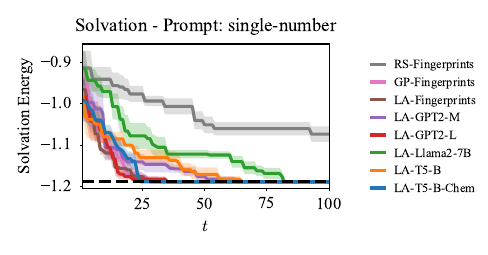}

	\includegraphics[width=0.45\linewidth]{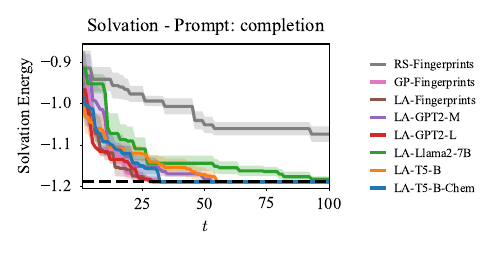}

	\vspace{-2em}
\end{figure}

\begin{summarybox}
	General LLMs---LLAMA2, GPT2, T5---are not good.
	Domain-specific LLM is required for good results.
\end{summarybox}

\clearpage

\section*{Finding 3: Effects of finetuning}

Finetuning: LoRA is applied to the attention layers (query, value) of the foundation model.

\begin{figure}[h!]
	\centering
	\includegraphics[width=0.5\linewidth]{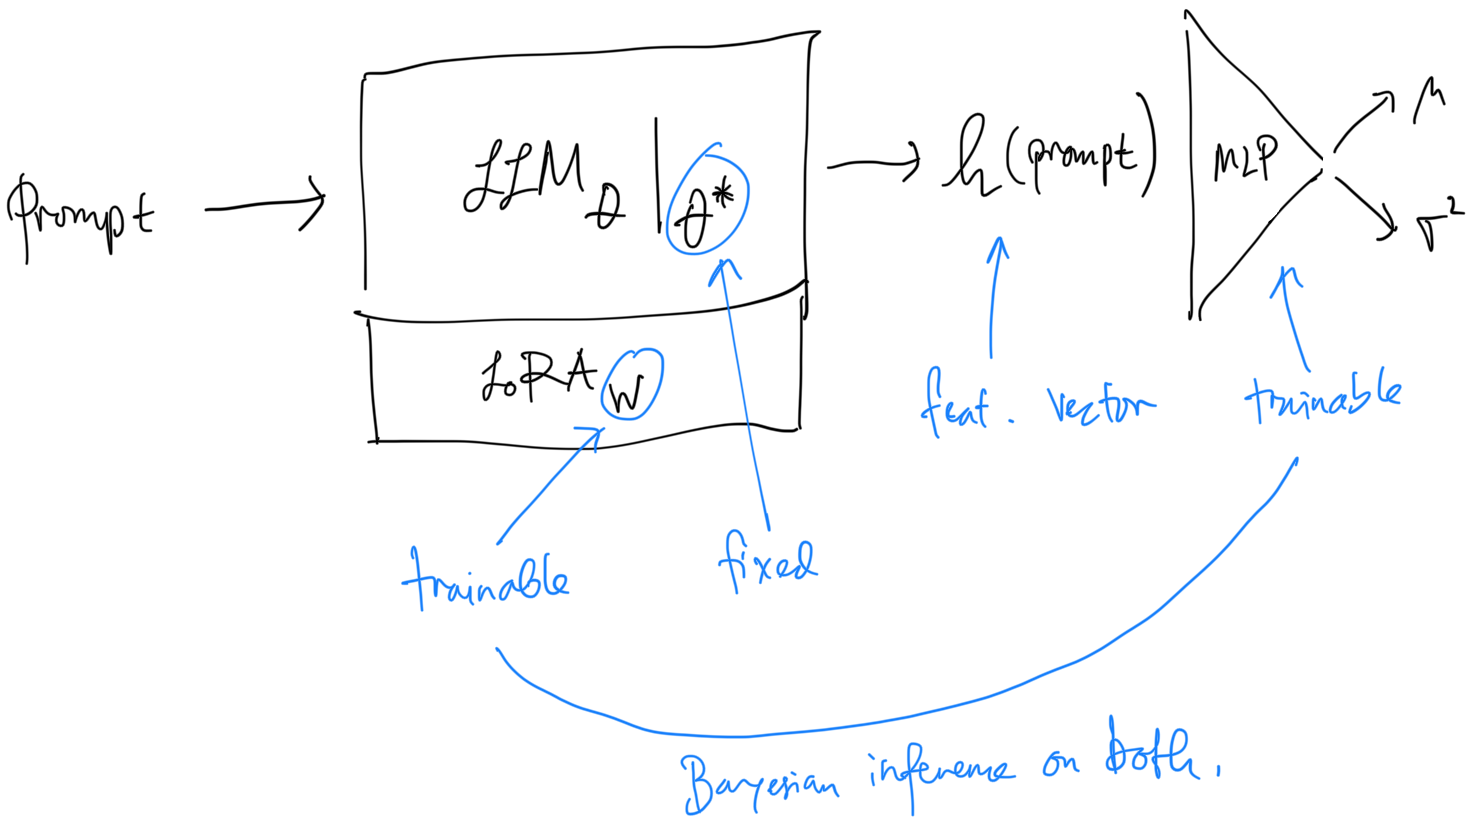}

	\caption{
		\textbf{Source of uncertainty:} Both the adapted LLM \& the regression head. (Via the Laplace approximation.)
	}
\end{figure}

\begin{figure}[h!]
	\centering

	\includegraphics[width=0.45\linewidth]{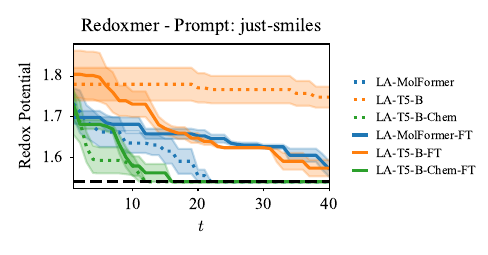}
	\includegraphics[width=0.45\linewidth]{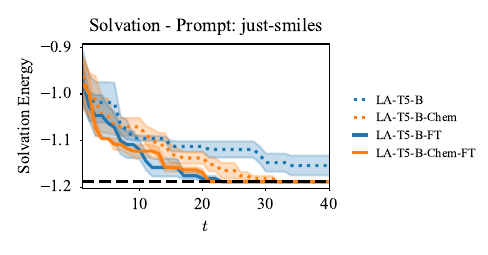}

	\caption{
		Finetuning performance. LoRA is used to adapt the LLM.
		The acquisition function is Thompson sampling.
	}
\end{figure}

\begin{summarybox}
	Additionally finetuning the LLM and taking into account the uncertainty of the finetuned LoRA weights \(\implies\) better results.
\end{summarybox}

\clearpage

\section*{Previous work}

\begin{itemize}
	\item Previous work, e.g.\ \citet{ramos2023bayesopticl,anonymous2023llambo} are using in-context learning (ICL).
	      \begin{itemize}
		      \item Prompting ChatGPT, e.g., \\
		            \emph{``I'm interested in estimating the redox potential of molecules, represented by their SMILES string. Here are some known data: \\
			            - SMILES: \texttt{\{smiles1\}}; redox potential: \texttt{\{redox1\}}, \\
			            - SMILES: \texttt{\{smiles2\}}; redox potential: \texttt{\{redox2\}}, \\
			            - SMILES: \texttt{\{smiles3\}}; redox potential: \texttt{\{redox3\}}. \\  Now, what is the estimated redox potential of \texttt{\{new\_smiles\}}?''}
	      \end{itemize}
	\item Their interpretation of \emph{Bayesian} optimization is quite ``liberal''
	      \begin{itemize}
		      \item \citet{ramos2023bayesopticl}: Using tokens' softmax probabilities as the uncertainty.
		      \item \citet{anonymous2023llambo}: The source of uncertainty is in the prompt templates. I.e., have \(k\) different prompts of the same data, then compute the variance of ChatGPT's answers.
	      \end{itemize}
	\item[] \(\implies\) They are just heuristic, and not principled BayesOpt methods.
	\item \textbf{Our goal:} Provide a way to do a principled BayesOpt with LLMs \& study our hypothesis.
\end{itemize}

\clearpage

\section*{Proposed story line}

\begin{enumerate}[(a)]
	\item \textbf{Motivation}
	      \begin{enumerate}[(i)]
		      \item LLMs seem useful for many task; their large sizes carry a lot of information. Might be useful as a prior for BayesOpt in molecular space.
		      \item From chemistry standpoint: \dots
		      \item Previous works are largely heuristic
	      \end{enumerate}
	\item \textbf{Contribution}
	      \begin{enumerate}[(i)]
		      \item Principled formulation of LLMs as surrogate functions in molecular BayesOpt.
		      \item A study of how the promises \& pitfalls of LLMs as surrogates.
		      \item Open source, easy to use implementation that accept any LLM
	      \end{enumerate}
	\item \textbf{Tentative messages/conclusions}
	      \begin{enumerate}[(i)]
		      \item Non-finetuned general LLMs are \emph{not} good as surrogates \(\implies\) raising questions of how reasonable are ICL-based methods
		            \begin{itemize}
			            \item (On top of them being unprincipled in terms of the uncertainty quantification.)
		            \end{itemize}
		      \item Domain-specific LLM is a good starting point. Finetuning generally improves performance.
		            \begin{itemize}
			            \item LLMs work actually because they have exposure to domain-related infos, i.e., standard transfer learning setup, not so much because of their ``intelligence''.
			            \item The above fit Occam's razor better; we verified empirically.
		            \end{itemize}
		      \item This is a good news: We don't need very large (expensive!) LLMs to get the best BayesOpt performance! T5-B-Chem is the smallest model here, only 220M params---everyone can do BayesOpt with LLMs!
		      \item Being Bayesian, in the LLM era, is not hard! No need for fancy yet kinda flawed uncertainty quantification heuristics.
	      \end{enumerate}
\end{enumerate}

\vfill\null

\subsection*{TO-DO:}
\begin{itemize}
	\item More baselines, esp.\ in-context learning \& GNN embedding.
	\item Evaluate on all datasets provided by Felix.
	\item Multi-objective optimization results.
\end{itemize}

\clearpage

\begin{figure*}
	\centering
	{\large \textbf{Redox-mer, t-SNE}}\par\vspace{1em}

	\begin{minipage}{0.24\textwidth}
		\includegraphics[width=\textwidth]{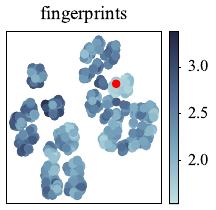}
	\end{minipage}
	\begin{minipage}{0.725\textwidth}
		\includegraphics[width=\textwidth]{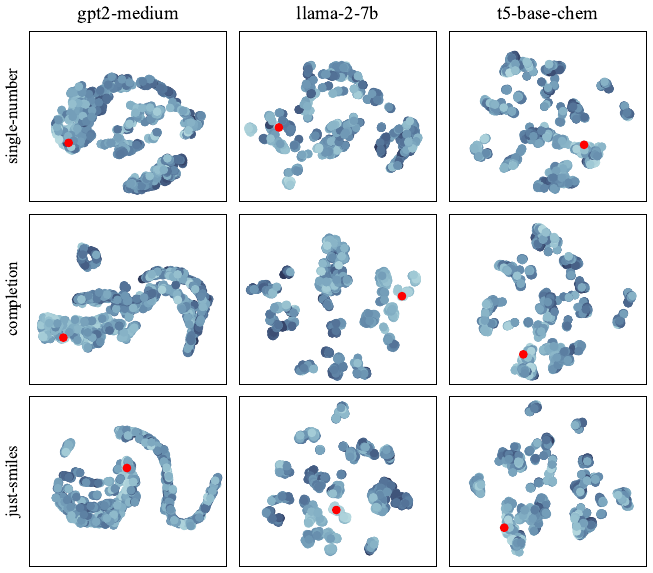}
	\end{minipage}

	\caption{
		t-SNE visualization of different embeddings (e.g., last hidden states of a LLM) for the \texttt{redox-mer} dataset.
		Red indicates the optimum.
		Rows indicate prompt types, columns indicate foundation models.
		The foundation model \textbf{t5-base-chem} is a chemistry-specific LLM by \citet{christofidellis2023unifying}.
		For prompt types,
		\textbf{just-smiles}: \emph{``\texttt{\{smiles\_str\}}''};
		\textbf{completion}: \emph{``The estimated redox potential of the molecule \texttt{\{smiles\_str\}} is: ''};
		\textbf{single-number}: \emph{``Answer with just numbers without any further explanation! What is the estimated redox potential of the molecule with the SMILES string \texttt{\{smiles\_str\}}?''}.
	}
\end{figure*}

\begin{figure*}
	\centering
	{\large \textbf{Redox-mer, UMAP}}\par\vspace{1em}

	\begin{minipage}{0.24\textwidth}
		\includegraphics[width=\textwidth]{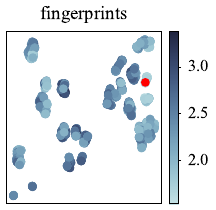}
	\end{minipage}
	\begin{minipage}{0.725\textwidth}
		\includegraphics[width=\textwidth]{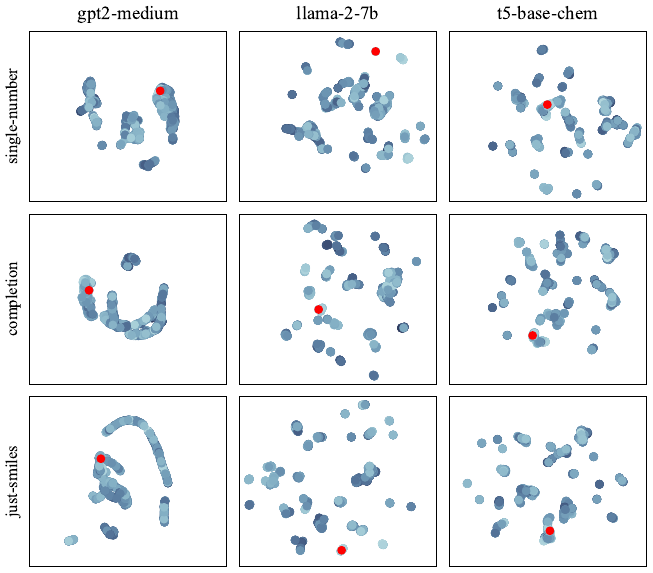}
	\end{minipage}

	\caption{
		UMAP visualization of different embeddings (e.g., last hidden states of a LLM) for the \texttt{redox-mer} dataset.
		Red indicates the optimum.
		Rows indicate prompt types, columns indicate foundation models.
		The foundation model \textbf{t5-base-chem} is a chemistry-specific LLM by \citet{christofidellis2023unifying}.
		For prompt types,
		\textbf{just-smiles}: \emph{``\texttt{\{smiles\_str\}}''};
		\textbf{completion}: \emph{``The estimated redox potential of the molecule \texttt{\{smiles\_str\}} is: ''};
		\textbf{single-number}: \emph{``Answer with just numbers without any further explanation! What is the estimated redox potential of the molecule with the SMILES string \texttt{\{smiles\_str\}}?''}.
	}
\end{figure*}

\begin{figure*}
	\centering
	{\large \textbf{Redox-mer, t-SNE, Average}}\par\vspace{1em}

	\begin{minipage}{0.24\textwidth}
		\includegraphics[width=\textwidth]{figs/redox-mer/dim_reduction/tsne_fingerprints}
	\end{minipage}
	\begin{minipage}{0.725\textwidth}
		\includegraphics[width=\textwidth]{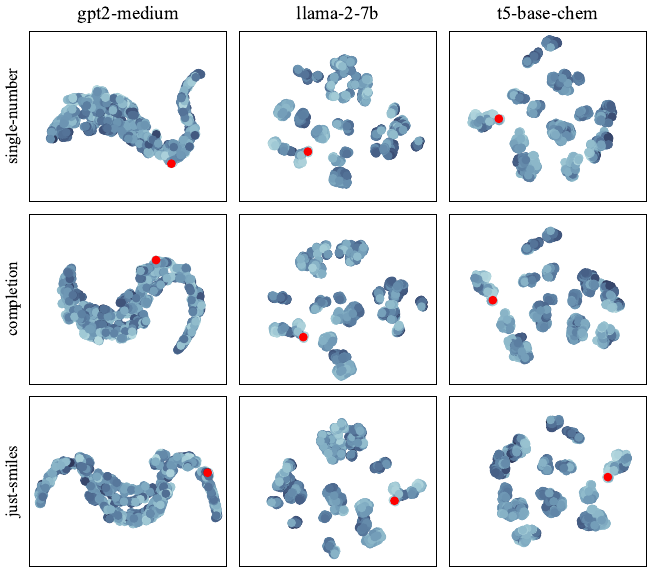}
	\end{minipage}

	\caption{
		t-SNE visualization of different embeddings (e.g., last hidden states of a LLM) for the \texttt{redox-mer} dataset.
		Red indicates the optimum.
		Rows indicate prompt types, columns indicate foundation models.
		The foundation model \textbf{t5-base-chem} is a chemistry-specific LLM by \citet{christofidellis2023unifying}.
		For prompt types,
		\textbf{just-smiles}: \emph{``\texttt{\{smiles\_str\}}''};
		\textbf{completion}: \emph{``The estimated redox potential of the molecule \texttt{\{smiles\_str\}} is: ''};
		\textbf{single-number}: \emph{``Answer with just numbers without any further explanation! What is the estimated redox potential of the molecule with the SMILES string \texttt{\{smiles\_str\}}?''}.
	}
\end{figure*}

\begin{figure*}
	\centering
	{\large \textbf{Redox-mer, UMAP, Average}}\par\vspace{1em}

	\begin{minipage}{0.24\textwidth}
		\includegraphics[width=\textwidth]{figs/redox-mer/dim_reduction/umap_fingerprints}
	\end{minipage}
	\begin{minipage}{0.725\textwidth}
		\includegraphics[width=\textwidth]{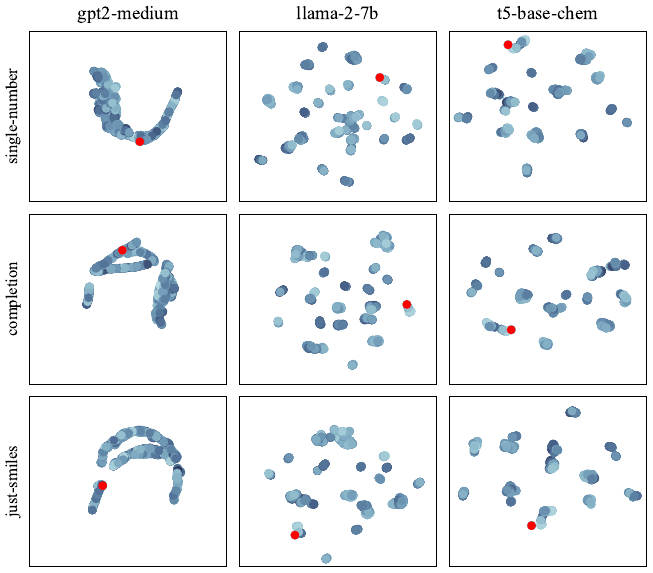}
	\end{minipage}

	\caption{
		UMAP visualization of different embeddings (e.g., last hidden states of a LLM) for the \texttt{redox-mer} dataset.
		Red indicates the optimum.
		Rows indicate prompt types, columns indicate foundation models.
		The foundation model \textbf{t5-base-chem} is a chemistry-specific LLM by \citet{christofidellis2023unifying}.
		For prompt types,
		\textbf{just-smiles}: \emph{``\texttt{\{smiles\_str\}}''};
		\textbf{completion}: \emph{``The estimated redox potential of the molecule \texttt{\{smiles\_str\}} is: ''};
		\textbf{single-number}: \emph{``Answer with just numbers without any further explanation! What is the estimated redox potential of the molecule with the SMILES string \texttt{\{smiles\_str\}}?''}.
	}
\end{figure*}
